# Supplementary material for: SmartMask: Context Aware High-Fidelity Mask Generation for Fine-grained Object Insertion and Layout Control
Source: arXiv:2312.05039 source file (2023-12-08)
Supplement: Supplementary file 1 [file smartmask-supp.tex]

%%%%%%%%% TITLE - PLEASE UPDATE
% \title{\textcolor{cvprblue}{MaskGen:} High Fidelity Layout Control with Sequential Layer Generation}
% \title{Supplementary Material \\ \textcolor{cvprblue}{SmartMask:} Context Aware High-Fidelity Mask Generation for \\Fine-grained Object Insertion and Layout Control}
% \title{\textcolor{cvprblue}{SmartMask:} Context Aware High-Fidelity Mask Generation for \\Fine-grained Object Insertion and Layout Control}

%%%%%%%%% AUTHORS - PLEASE UPDATE
\author{}

\appendix
% \maketitle
\maketitlesupplementary

%%%%%%%%% BODY TEXT
% \newpage
\section{Additional Results}
\label{sec:additional-results}

In this section, we include some  additional results which could not be included due to space constraints in the main paper. In particular, we demonstrate the ability of our approach to perform context-aware multi-object insertion in Sec.~\ref{sec:multi-object-insertion}.
We also show additional results using \Smask for object insertion with better background preservation in Sec.~\ref{sec:single-object-insertion}.  We provide additional results analysing the ability of our model to perform mask-free insertion in Sec.~\ref{sec:mask-free object-insertion}. Finally, we include additional results comparing our output mask quality with SmartBrush mask-head outputs \cite{xie2023smartbrush} and various Inpaint+HQSAM methods in Sec.~\ref{sec:output-mask-quality}.

\subsection{SmartMask for Multiple Object Insertion}
\label{sec:multi-object-insertion}

\begin{figure*}[h!]
\vskip -0.15in
\begin{center}
\centerline{\includegraphics[width=1.\linewidth]{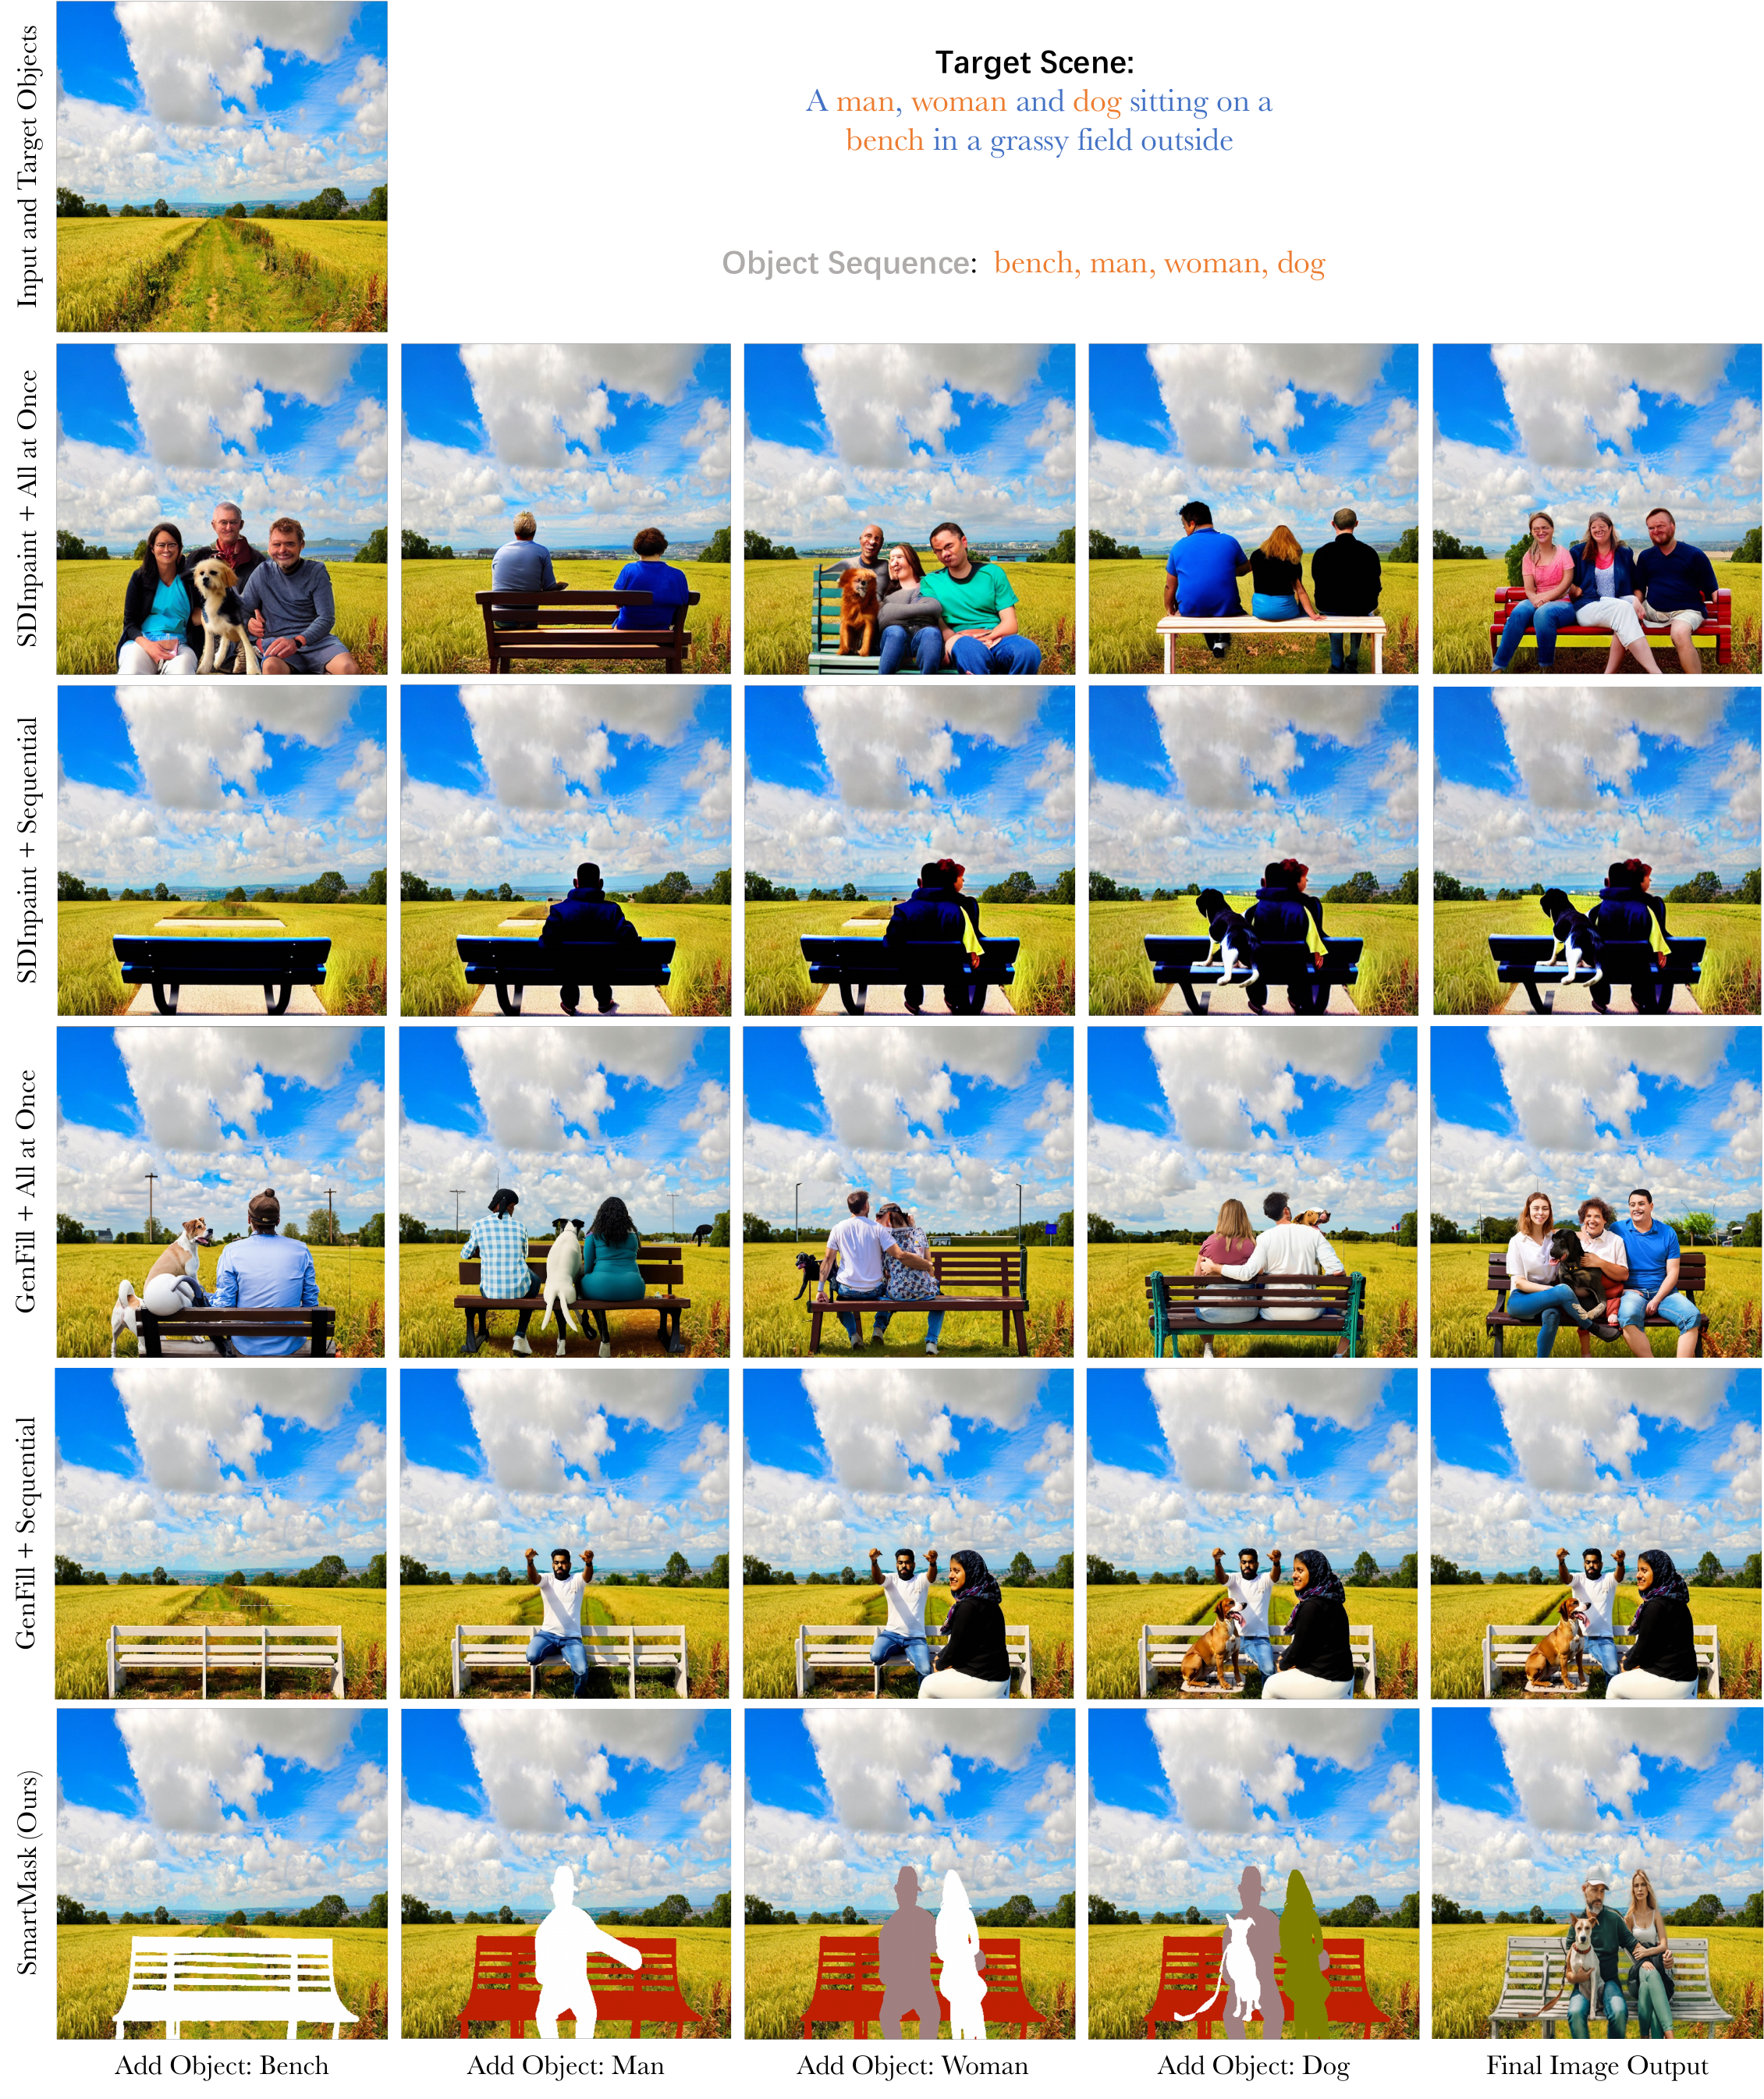}}
\vskip -0.1in
\caption{\emph{\textbf{SmartMask for multi-object insertion.}} We observe that prior state-of-the-art image inpainting methods \cite{rombach2021highresolution,adobe2023firefly} either lead to 1) incorrect objects (\bline{missing dog}) or visual-artifacts (\eg, \bline{people facing bench's back})  when adding all objects at once (row-2, row-4), or, 2) introduce inconsistency-artifacts (\eg, \bline{woman and dog in front of bench} in row-3, \bline{dog and woman not sitting on same bench} in row-5) when adding objects sequentially.  Furthermore, the generated objects (\bline{man, woman and dog} in row-5) can appear non-interacting when generated in a sequential manner.
\Smask helps address this by allowing the user to first add a coherent sequence of context-aware object masks, before using SDXL-based-ControlNet-Inpaint \cite{zhang2023adding,diffusers} model to perform precise object insertion for multiple objects.}
\label{fig:multi-obj-insertion-v1}
\end{center}
\vskip -0.4in
\end{figure*}

\begin{figure*}[h!]
% \vskip -0.15in
\begin{center}
\centerline{\includegraphics[width=1.\linewidth]{assets/multi-obj-insertion-p1-v6.pdf}}
\vskip -0.1in
\caption{\emph{\textbf{SmartMask for multi-object insertion.}} We observe that prior state-of-the-art image inpainting methods \cite{rombach2021highresolution,adobe2023firefly} either lead to incorrect objects (row-2, row-4) when adding all objects at once, or, introduce artifacts (\eg \bline{woman} in row-3, \bline{man's face} and \bline{woman's dress} in row-5) when adding objects sequentially.  \Smask helps address this by allowing the user to first add a sequence of context-aware object masks, before using SDXL-based-ControlNet-Inpaint \cite{zhang2023adding,diffusers} model to perform precise object insertion for multiple objects.}
\label{fig:multi-obj-insertion-v2}
\end{center}
\vskip -0.4in
\end{figure*}

While adding a single object to an input image is useful, in practical applications users would typically want to add multiple objects to the input image 
% in a coherent manner 
in order to obtain a desired output scene. For instance, given an image depicting a grassy field, the user may wish to add multiple objects \{\bline{bench, man, woman, dog}\} such that the final scene aligns with the context \bline{`a couple with their dog sitting on a bench in a grassy field'} (Fig.~\ref{fig:multi-obj-insertion-v1}). In this section, we show that unlike prior works which are limited to adding each object independently, the proposed approach allows the user to perform multiple-object insertion in a context-aware manner.

Results are shown in Fig.~\ref{fig:multi-obj-insertion-v1}, \ref{fig:multi-obj-insertion-v2}. In particular, we show comparisons with prior inpainting methods when \emph{a)} all objects (\eg bench, man, woman, dog in Fig.~\ref{fig:multi-obj-insertion-v1}) are inserted all at once, and \emph{b)} different objects are inserted in a sequential manner. We observe that when inserting all objects at once, prior works typically lead to 1) incorrect/missing objects (\eg missing dog, additional person in Fig.~\ref{fig:multi-obj-insertion-v1}), or, 2) introduce visual-artifacts (\eg, \emph{people facing bench's back}). On the other hand, when adding different objects in sequential manner, we observe that prior works often lead to inconsistency-artifacts. For instance, when adding the \{\bline{bench, man, woman, dog}\} in Fig.~\ref{fig:multi-obj-insertion-v1}, we observe that SD-Inpaint \cite{rombach2021highresolution} leads to outputs which put the \emph{woman and dog on back of the bench}. Commercial state-of-the-art Adobe GenFill \cite{adobe2023firefly} performs better however 
% since each object is added in an independent manner, 
the \emph{dog and woman do not appear to be sitting on the same bench as man}. Furthermore, the generated objects (\bline{man, woman and dog} in row-5) can appear non-interacting when generated in a sequential manner. \Smask helps address this by allowing the user to first add a coherent sequence of context-aware object masks, before using SDXL-based-ControlNet-Inpaint \cite{zhang2023adding,diffusers} model to perform precise object insertion.

A similar observation is also found in in Fig.~\ref{fig:multi-obj-insertion-v2}, where we see that prior inpainting methods \cite{rombach2021highresolution,adobe2023firefly} either lead to (a) incorrect objects (\eg, missing child, additional person) when adding all objects at once, or, (b) introduce artifacts (\eg \bline{woman} in row-3, \bline{man's face} and \bline{woman's dress} in row-5) when adding objects sequentially. Furthermore, the object insertion is done in a context-unaware manner. For instance, when adding \bline{flowers} near the hand of the child in row-5, we observe that Adobe GenFill \cite{adobe2023firefly} simply adds a big-flower around the hand region. In contrast, the context-aware ability of \Smask model allows it to add the flowers as a bouquet which is held by the child, thereby allowing more coherent multi-object insertion over prior works.

\subsection{Additional Results for Single Object Insertion}
\label{sec:single-object-insertion}

\begin{figure*}[h!]
% \vskip -0.15in
\begin{center}
\centering
     \begin{subfigure}[b]{1.\textwidth}
         \centering
         \includegraphics[width=\textwidth]{assets/inpainting-additional-p1-v3.pdf}
         \vskip -0.05in
         % \caption{\emph{Mask-free object insertion}}
         % \label{fig:guid-}
     \end{subfigure}
     % \hfill
     % \vskip -0.19in  
     \begin{subfigure}[b]{1.\textwidth}
         \centering
         \includegraphics[width=\textwidth]{assets/inpainting-additional-p2-v4.pdf}
         \vskip -0.05in
         % \caption{\emph{Mask-free object insertion}}
         % \label{fig:guid-}
     \end{subfigure}
% \centerline{\includegraphics[width=1.\linewidth]{assets/ipainting-vis-v1-dummy.pdf}}
\vskip -0.1in
\caption{\emph{\textbf{Additional Results for Single Object-Insertion.}} We observe that as compared to
with state-of-the-art image inpainting \cite{xie2023smartbrush,rombach2021highresolution,podell2023sdxl,avrahami2023blended} methods, \Smask allows the user to perform object insertion while better preserving the background around the inserted object. }
\label{fig:additional-results-single-insertion}
\end{center}
\vskip -0.4in
\end{figure*}

In this section, we include additional results on using \Smask for single-object insertion across diverse object categories.
% We also include additional qualitative comparisons against SDXL-Inpaint \cite{podell2023sdxl} and Gligen-Inpaint \cite{li2023gligen}.
Results are shown in Fig.~\ref{fig:additional-results-single-insertion}. Similar to the results in the main paper, we find that prior image inpainting methods typically lead to huge changes in the image background when adding new objects. For instance, when adding \bline{child to a birthday party scene} (row-1, Fig.~\ref{fig:additional-results-single-insertion}), we observe that prior works completely remove the background table with birthday decorations. In contrast, the proposed approach is able to generate scene-aware masks which can interact with already existing objects in the input image. This allows it to place the child as if sitting on the table in the original image.

We also observe that the effect of compromised backgroud preservation is even more severe when adding new objects near already existing humans in the input image. For instance, in row-4 (Fig.~\ref{fig:additional-results-single-insertion}) we observe that when adding a \bline{woman} next to a man sitting on top of mountain rock, prior inpainting works \eg, SDInpaint, SDXL-Inpaint\cite{rombach2021highresolution,podell2023sdxl} either convert the man himself to a woman, or, add two woman on the image which replace the man altogether. This is clearly undesirable if the user simply wants a final scene with a couple sitting on top of a mountain rock. \Smask helps address this by first predicting a precise object mask for adding the woman on the side of the man, before then using ControlNet-Inpaint \cite{diffusers, zhang2023adding} model for precise object insertion without affecting the image regions for the man.

\subsection{Mask-free Object Insertion}
\label{sec:mask-free object-insertion}
% show cases e.g. adding car in front of house where the standard inpainting methods either do not add anything, or add objects at wrong scale. using mask-free insertion can instead suggest better scale and position for object insertion.
A key advantage of \Smask is that unlike prior works which rely on a user-provided coarse mask, the proposed approach can also be used without user-mask guidance. This allows \Smask to facilitate mask-free object insertion, where it automatically 
provides diverse suggestions for inserting the target-object in the input image.
% generates diverse scene-aware precise object masks for inserting the target object in the input image.

Results are shown in Fig.~\ref{fig:mask-free-insertion-v1}, Fig.~\ref{fig:mask-free-insertion-v2}.  We observe that unlike prior image-inpainting methods which rely on user-provided masks for determining object location and scale, \Smask also allows for \emph{mask-free object insertion}. This allows the user to generate diverse object insertion suggestions for putting the target object (\eg, \bline{ship} in row-1 Fig.~\ref{fig:mask-free-insertion-v1}, \bline{chair} in row-5 Fig.~\ref{fig:mask-free-insertion-v2}) in the input image at different positions and scales. We also observe that the masks are generated in a scene-aware manner, and can therefore account for the existing scene elements when adding the new object. For instance, when adding \bline{man on bed} in row-5 Fig.~\ref{fig:mask-free-insertion-v1}, we observe that model autoamtically predicts diverse suggestions where the man is sitting or lying down on the bed in diverse poses. Similarly, when adding \bline{a car riding down the mountain road} in row-3 Fig.~\ref{fig:mask-free-insertion-v1}, the car is positioned at correct pose and angle on the road region, despite the turning and slanted nature of the road. Similarly, when adding \bline{a lamp to a living room} in Fig.~\ref{fig:mask-free-insertion-v2}, we observe that \Smask is able to understand the scene-geometry and is able to provide diverse suggestions for positioning the lamp both on the floor and the background cabinets. 

Finally, we also observe that the object insertion suggestions are generated at different scales depending on the position within the input image. Thus, objects close to camera are added through larger masks while objects away from camera are generated using smaller masks (\eg, \bline{adding a motorbike parked beside a car} in row-4 Fig.~\ref{fig:mask-free-insertion-v2}).

\begin{figure*}[h!]
\vskip -0.15in
\begin{center}
\centerline{\includegraphics[width=1.\linewidth]{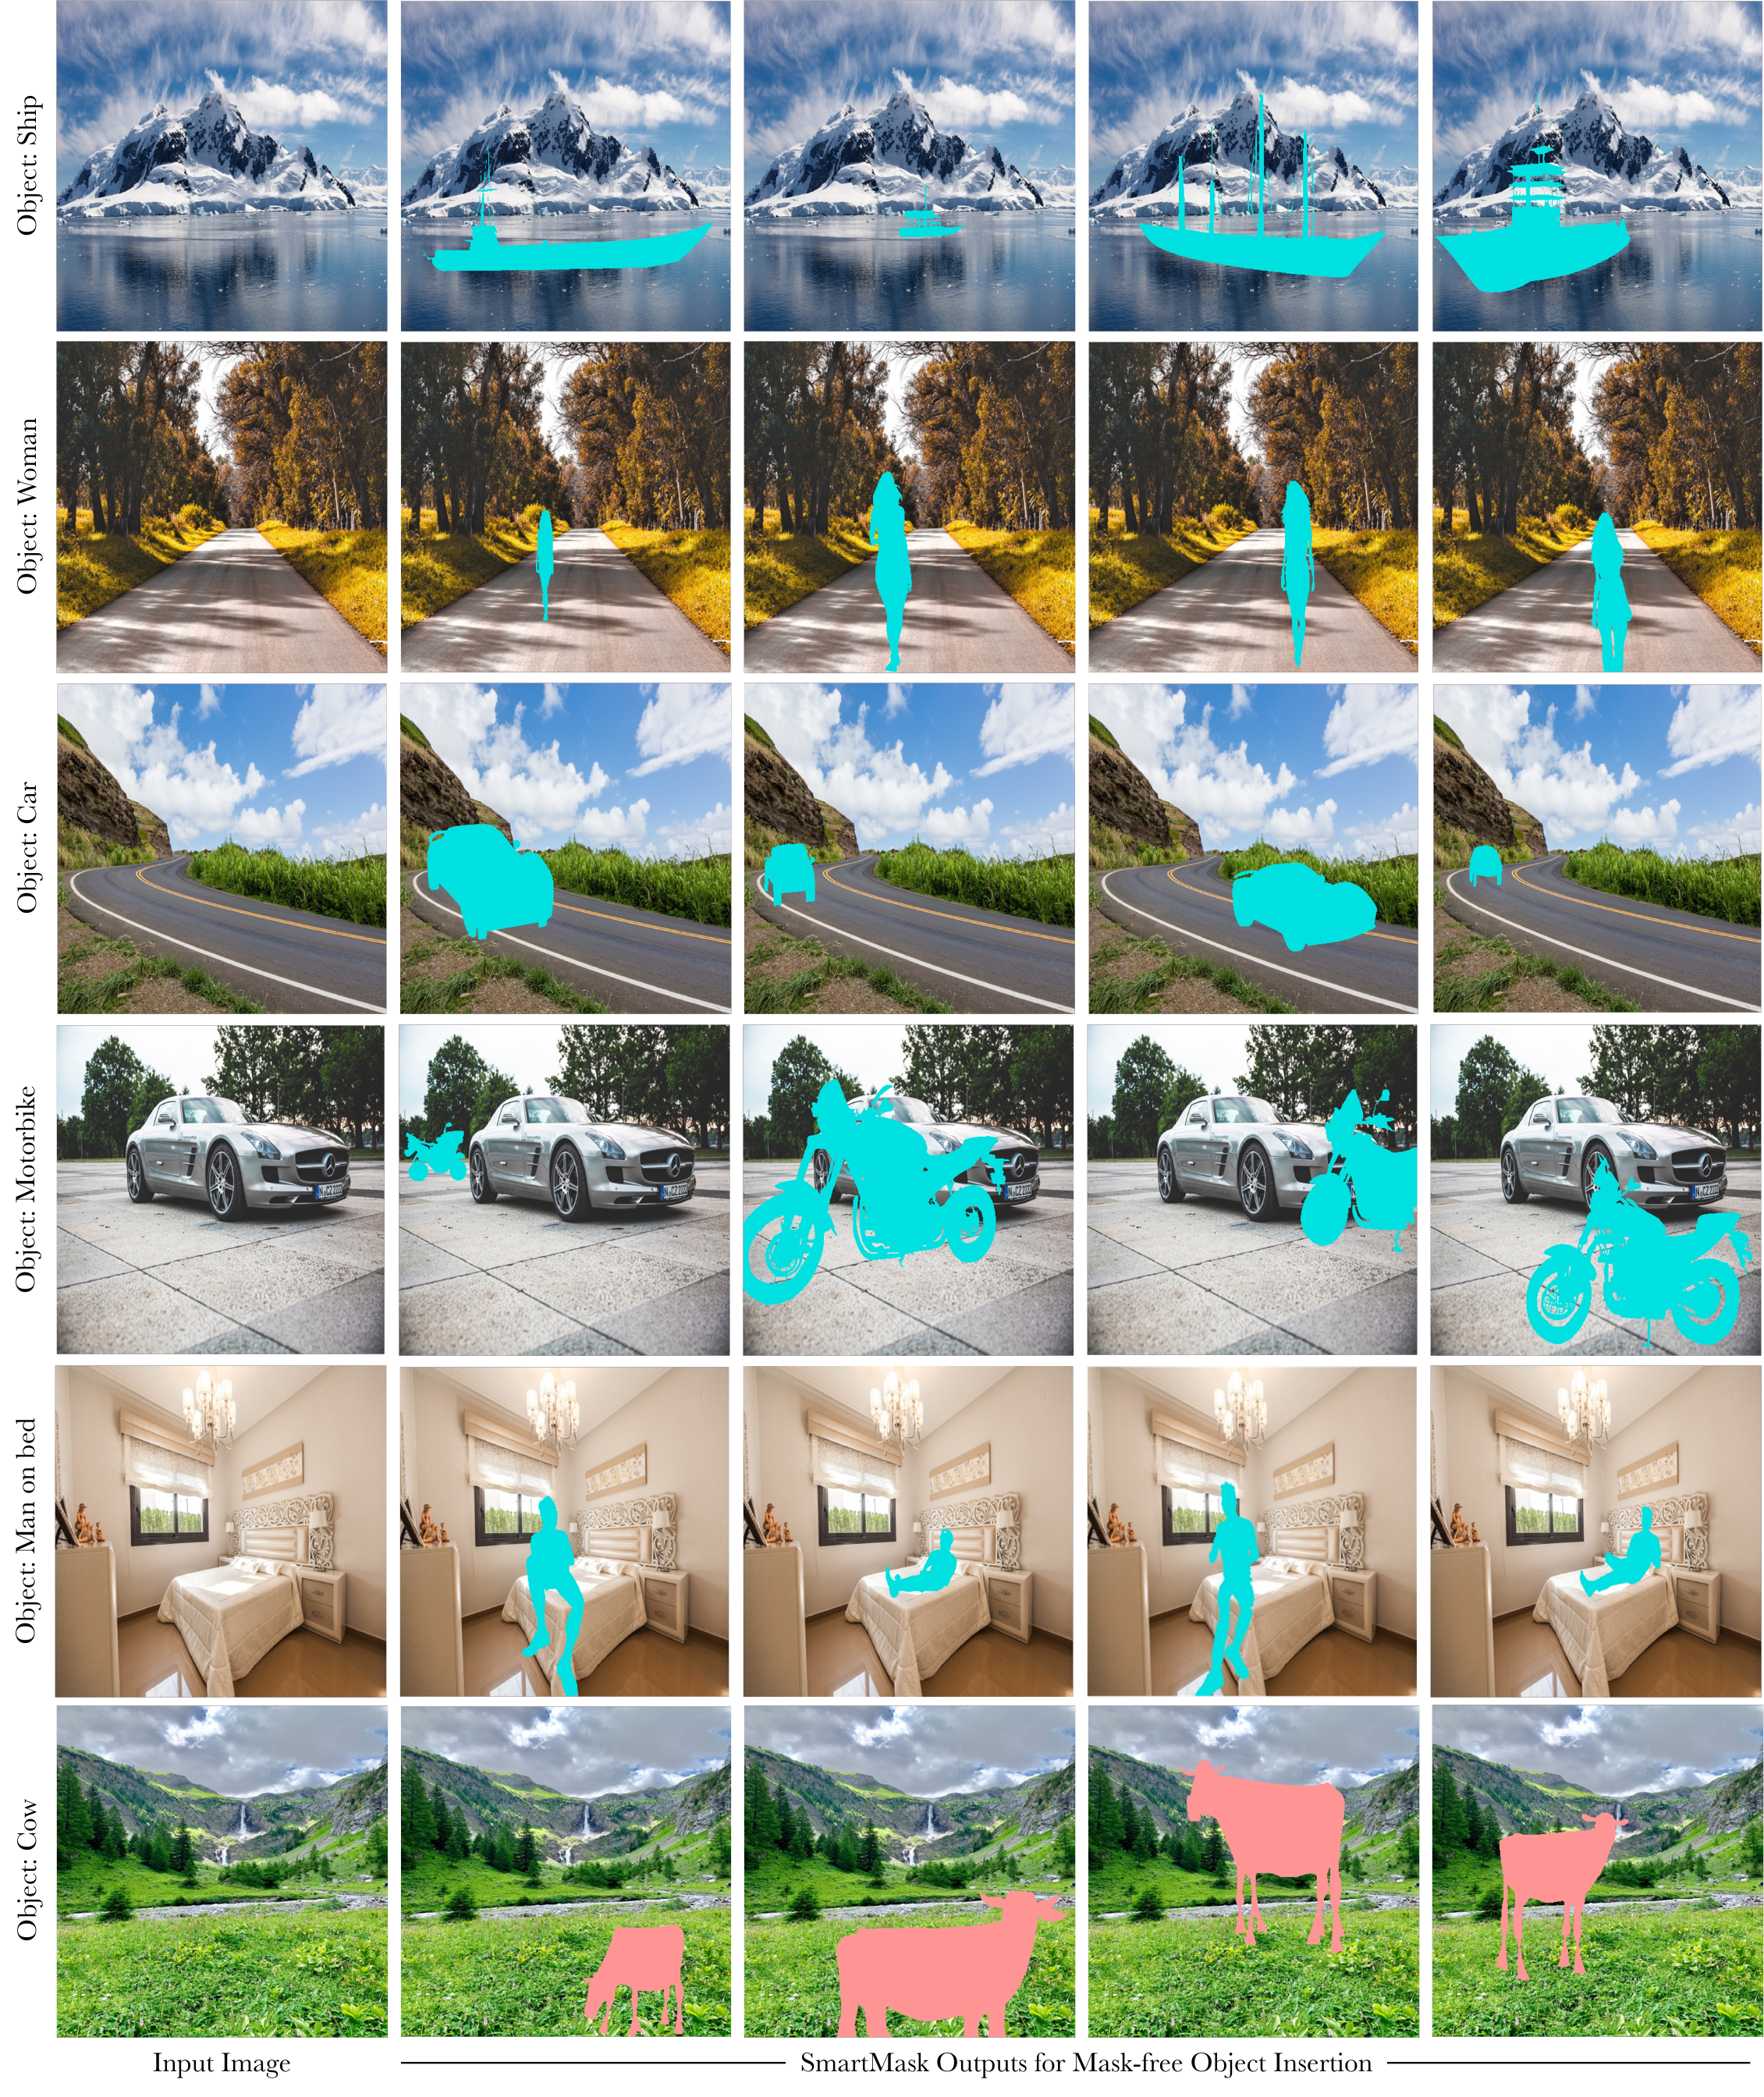}}
\vskip -0.1in
\caption{\emph{\textbf{SmartMask for mask-free object insertion.}} We observe that unlike prior image-inpainting methods which rely on user coarse masks for object location and scale, \Smask also allows for \emph{mask-free object insertion}. This allows the user to generate diverse object insertion suggestions for putting the target object (\eg, \bline{ship}) in the input image at different positions and scales. Note that the masks are generated in a scene-aware manner, and can therefore account for the existing scene elements (\eg, \bline{man lying on bed} in row-5, \bline{car riding down the road} in row-3 \etc). Also notice that the object insertion suggestions are generated at different scales: thus objects close to camera are larger and away from camera are smaller (\eg, \bline{motorbike parked beside a car} in row-4).}
\label{fig:mask-free-insertion-v1}
\end{center}
\vskip -0.4in
\end{figure*}

\begin{figure*}[h!]
\vskip -0.15in
\begin{center}
\centerline{\includegraphics[width=1.\linewidth]{assets/mask-free-insertion-p2-v1.pdf}}
\vskip -0.1in
\caption{\emph{\textbf{SmartMask for mask-free object insertion.}} We observe that unlike prior image-inpainting methods which rely on user coarse masks for object location and scale, \Smask also allows for \emph{mask-free object insertion}. This allows the user to generate diverse object insertion suggestions for putting the target object (\eg, \bline{bench} in row-1, \bline{dog} in row-6) in the input image at different positions and scales. Note that the masks are generated in a scene-aware manner, and can therefore account for the existing scene elements (\eg, \bline{lamp in living room} in row-4, \bline{chair} at different empty positions in row-5 \etc). Also notice that the object insertion suggestions are generated at different scales: thus objects close to camera are larger and away from camera are smaller (\eg, \bline{child near a waterfall} in row-2).}
\label{fig:mask-free-insertion-v2}
\end{center}
\vskip -0.4in
\end{figure*}

\begin{figure*}[h!]
% \vskip -0.15in
\begin{center}
\centerline{\includegraphics[width=1.\linewidth]{assets/mask-quality-comp-p1-v2.pdf}}
% \vskip -0.1in
\caption{\emph{\textbf{Analysing output mask quality.}} 
We observe that SmartBrush mask-head predictions \cite{xie2023smartbrush} and Inpaint+HQSAM outputs (\ie,  inpainting first and then using HQSAM \cite{sam_hq} typically lead to coarse masks for the target object. Furthermore, the generated masks can often have artifacts in the target regions. In contrast,  \Smask is able to generate diverse mask suggestions with more finegrain details (e.g., \bline{women details} in example-1, \bline{tree structure} in example-2) for inserting the target object in the original image.
}
\label{fig:mask-quality-comp-v1}
\end{center}
\vskip -0.2in
\end{figure*}

\begin{figure*}[h!]
% \vskip -0.15in
\begin{center}
\centerline{\includegraphics[width=1.\linewidth]{assets/mask-quality-comp-p2-v2.pdf}}
% \vskip -0.1in
\caption{\emph{\textbf{Analysing output mask quality.}} 
We observe that SmartBrush mask-head predictions \cite{xie2023smartbrush} and Inpaint+HQSAM outputs (\ie,  inpainting first and then using HQSAM \cite{sam_hq} typically lead to coarse masks for the target object. Furthermore, the generated masks can often have artifacts in the target regions. In contrast,  \Smask is able to generate diverse mask suggestions with more finegrain details (e.g., \bline{living room chair} in example-1, \bline{dog details} in example-2) for inserting the target object in the original image.
}
\label{fig:mask-quality-comp-v2}
\end{center}
\vskip -0.2in
\end{figure*}

\begin{figure*}[h!]
% \vskip -0.15in
\begin{center}
\centerline{\includegraphics[width=1.\linewidth]{assets/inpaint-hqsam-comp-v1.pdf}}
% \vskip -0.1in
\caption{\emph{\textbf{Limitation of Inpaint + HQSAM.}} In addition to poor quality mask outputs (refer Fig. \ref{fig:mask-quality-comp-v1}, \ref{fig:mask-quality-comp-v2}), we observe that Inpaint+HQSAM methods (\ie inpainting first and then using HQSAM to obtain target object masks) can also
lead to scene-unaware masks. For instance, we observe that when inpainting the target object (\ie \bline{woman}) in the bounding box area, Adobe SmartBrush \cite{xie2023smartbrush} modifies the background to also add a chair (row-2). The use of HQSAM \cite{sam_hq} on the inpainted outputs thus leads to masks which portray the woman as sitting in the air in the original image (row-3). In contrast, we observe that \Smask is able to generate better quality scene-aware masks for inserting the target object where the \bline{woman is either sitting on the floor} or \bline{standing in the provided mask area}.
}
\label{fig:inpaint-hqsam-limitation}
\end{center}
% \vskip -0.4in
\end{figure*}

\subsection{Additional Results on Output Mask Quality}
\label{sec:output-mask-quality}

We also report additional results comparing output mask quality with Smartbrush \cite{xie2023smartbrush} mask head which also predicts an object mask for the inserted object in addition to the inpainted output. Furthermore, we also compare the performance of \Smask generated masks with Inpaint + HQSAM methods when user bounding-box guidance is present. To this end, given an input image, object description and bounding-box mask, we first use an inpainting method \eg Adobe SmartBrush \cite{xie2023smartbrush} in order to inpaint the target object in the scene. The inpainted image output and corresponding bounding box are then used as input to the recently proposed HQ-SAM \cite{sam_hq} model in order to obtain segmentation masks for the target object.

Results are shown in Fig.~\ref{fig:mask-quality-comp-v1}, \ref{fig:mask-quality-comp-v2}. We observe that SmartBrush mask head \cite{xie2023smartbrush} only generates very coarse masks for the target object during inpainting. Furthermore, the SmartBrush masks often have artifacts \eg, \bline{woman} in Fig.~\ref{fig:mask-quality-comp-v1} and \bline{living room chair in} Fig.~\ref{fig:mask-quality-comp-v2}. Passing the output of the SmartBrush inpainting to HQ-SAM \cite{sam_hq} instead generates more finer quality masks. However, the generated masks are still fairly coarse and still have noticeable artifacts. For instance, when adding a tree to an outdoor scene with a lake (Fig.~\ref{fig:mask-quality-comp-v1}), we observe that SmartBrush + HQSAM generates very coarse masks for the tree region. In contrast, \Smask is able to generate significantly more detailed and diverse masks for the target object (\bline{tree}). Similarly, even when adding a \bline{living room chair} to a living room scene (refer Fig.~\ref{fig:mask-quality-comp-v2}), we observe that SmartBrush + HQSAM masks typically add very coarse masks for the target chair/couch. In contrast, \Smask is able to generate diverse variations with more finegrain details \eg, chair structure, pose, style \etc for inserting the target object in the original image.

In addition to poor quality mask outputs (refer Fig. \ref{fig:mask-quality-comp-v1}, \ref{fig:mask-quality-comp-v2}), we observe that Inpaint + HQSAM methods (\ie inpainting first and then using HQSAM to obtain target object masks) can also
lead to scene-unaware masks (refer Fig.~\ref{fig:inpaint-hqsam-limitation}). For instance, in Fig.~\ref{fig:inpaint-hqsam-limitation} we observe that when inpainting the target object (\ie \bline{woman}) in the bounding box area, Adobe SmartBrush \cite{xie2023smartbrush} modifies the background to also add a chair (row-2). The use of HQSAM \cite{sam_hq} on the inpainted outputs thus leads to masks which portray the woman as sitting in the air in the original image (row-3). In contrast, we observe that \Smask is able to generate better quality scene-aware masks for inserting the target object where the \bline{woman is either sitting on the floor} or \bline{standing in the provided mask area}, thereby facilitating better object insertion performance.

%-------------------------------------------------------------------------
% \newpage
\section{Experiment Details}
\label{sec:experiment-results}

In this section, we provide further information regarding the implementation of our approach 
% \eg, data preparation, training \etc 
(refer App.~\ref{sec:implementation-details})  as well as additional details on quantitative experiments used while reporting results in the main paper (refer App.~\ref{sec:quantitative-experiments}).

\subsection{Implementation details}
\label{sec:implementation-details}

\textbf{Data Preparation for Mask-Free Insertion.} 
The key idea of \Smask is to leverage semantic amodal segmentation datasets in order to obtain high-quality paired training annotations for mask-free object insertion. 
During training, given an image $\mathcal{I}$, with a sequence of ordered amodal semantic instance maps $\{A_1, A_2 \dots A_n\}$ and corresponding semantic object labels $\{\mathcal{O}_1, \mathcal{O}_2 \dots \mathcal{O}_n\}$, we first compute an intermediate layer semantic map as,
\begin{align}
    S_k = f_{layer}(\{A_1, A_2 \dots A_k\}) \quad where \ k \in [1,n]. \label{eq:intermediate-layer}
\end{align}
where $k$ is randomly chosen from $[1,n]$ and $f_{layer}$ is a layering operation which stacks the amodal semantic segmentation maps from $i \in [1,k]$ in an ordered manner (please refer Fig.~\textcolor{red}{2} main paper) as follows,
\begin{align*}
f_{layer}(A_1, A_2, \dots, A_k) = \bigoplus_{i=1}^{k} A_i \odot h(\mathcal{O}_i) \quad \text{for} \ i \in [1,k] \label{eq:layering-operation}
\end{align*}
where $\bigoplus$ represents the stacking operation and  $h(\mathcal{O}_i)$ is the \emph{rgb} encoding for the corresponding object description $\mathcal{O}_i$.
The \Smask model $\mathcal{D}_{\theta}$ is then trained to as input the above computed intermediate semantic layer map $S_k$, semantic description for next object $\mathcal{T}_{obj} \leftarrow \mathcal{O}_{k+1}$,  overall caption $\mathcal{T}_{context} \leftarrow C_\mathcal{I}$ (for image $\mathcal{I}$ computed using InstructBLIP \cite{instructblip}) and learns to predict the mask $\mathcal{M}_{obj}$ for the next object $\mathcal{O}_{k+1}$ as,
\begin{align}
    \mathcal{M}^{pred}_{obj} =  \mathcal{D}_{\theta} ( \mathcal{E}_{\phi}(\mathcal{S}_I), \mathcal{T}_{obj}, \mathcal{T}_{context}),\\
   s.t. \quad  \mathcal{M}^{gt}_{obj} = S_k \odot (1-A_{k+1}) + A_{k+1}
\end{align}
where the ground-truth model output $\mathcal{M}^{gt}_{obj}$
is modelled as the target object mask $A_{k+1}$ stacked on top of input map $S_k$ which helps provide the model better spatial context for target mask generation during the reverse diffusion process.

\textbf{Data Augmentation for Mask Control}. In addition to mask-free object insertion, \Smask also allows the user to provide an additional guidance input $\mathcal{G}_{obj}$ to control the better details of the output mask. During training, this is achieved through a simple data-augmentation strategy which randomly replaces input $S_k$ to \Smask as,
\begin{align}
    \Tilde{S_k} = g(S_k,G_{obj}) =  S_k \odot (1 - \alpha \ G_{obj})  +  \alpha \  G_{obj}, \label{eq:data-aug}
\end{align}
where $G_{obj}$ is the additional guidance input (\eg, bounding box mask, coarse scribbles \etc) provided by the user and $\alpha=0.7$ helps add additional guidance while still preserving the content of the original input $S_k$ after data augmentation.

In this paper, we mainly consider four main guidance inputs $G_{obj}$ for additional mask control at training time. \emph{1) Mask-free guidance:} $G_{obj} = \mathbf{0}^{H,W}$ which prompts the model to suggest fine-grained masks for object insertion at diverse
positions and scales.  \emph{2) Bounding-box guidance:} we set $G_{obj}$ as a binary mask corresponding to bounding-box for target object mask $A_{k+1}$. \emph{3) Coarse Spatial Guidance:} Given bounding coordinates $\mathbf{b}_{k+1} = \{x_{min},y_{min},x_{max},y_{max}\}$ for the  target object mask $A_{k+1}$, we first compute a randomly perturbed bbox location as,
\begin{align}
    \Tilde{\mathbf{b}}_{k+1} \leftarrow \mathbf{b}_{k+1} + \mathbf{p}_{k+1}, where \quad \mathbf{p}_{k+1} \in \mathbf{R}^4 
\end{align}
where $\mathbf{p}_{k+1} \sim U[-20,20]$ is sampled from a uniform distribution, and randomly perturbs the original bounding box $\mathbf{b}_{k+1}$. The guidance input $G_{obj}$ is then computed by applying a Gaussian-blur operation to a binary bounding-box mask for the perturbed bounding-box coordinates $\Tilde{\mathbf{b}}_{k+1}$

\emph{4) User scribbles:} Finally, we also allow the user to describe target object using free-form coarse scribbles, by setting $G_{obj}$ as the output of multi-scale morphological dilation operation applied on target object mask $A_{k+1}$.

\textbf{SmartMask Training.} 
In order to leverage the rich generalizable prior of T2I diffusion models,
we use the weights from publicly available Stable-Diffusion-v1.5 model \cite{rombach2021highresolution} in order to initialize the weights of the \Smask U-Net model. Similar to \cite{brooks2023instructpix2pix}, we modify the architecture of the U-Net model to also condition the output mask predictions on segmentation layout $\mathcal{S}_I$. The object description input $\mathcal{T}_{obj}$ and final-scene context  $\mathcal{T}_{context}$ are jointly fed to the diffusion model by modifying the input text tokens as follows,
\begin{align}
    \tau_{text} = \text{CLIP}(\mathcal{T}_{obj}) + \texttt{<sep>} + \text{CLIP}(\mathcal{T}_{context}),
\end{align}
where $\texttt{<sep>}$ is the separation token and $\text{CLIP}(\mathcal{T}_{obj})$, $\text{CLIP}(\mathcal{T}_{context})$ represents the CLIP tokens for the object-description $\mathcal{T}_{obj}$ and scene-context $\mathcal{T}_{context}$ respectively. The overall \Smask model is then trained for a total of 100k iterations with a batch size of 192 and learning rate $1e-5$ using 8 Nvidia-A100 GPUs.

\textbf{SmartMask Inference.} During inference, a panoptic semantic segmentation model finetuned on the dataset in Sec.~\textcolor{red}{4} of main paper is used for converting real image $\mathcal{I}$  to its semantic layout $\mathcal{S}_I$. The semantic layout $\mathcal{S}_I$ along with object description and scene context are used as input to \Smask model followed by a thresholding operation to obtain the target object mask. Finally, a ControlNet-Inpaint \cite{zhang2023adding,diffusers} model trained with SDXL backbone is used to perform precise object insertion with SmartMask outputs.

\textbf{Global Planning Model.} The global planning model (Sec.~\textcolor{red}{3.3} main paper) directly follows the visual-instruction tuning architecture from \cite{liu2023visual}. In particular, we use the recently proposed instruction-following \emph{vicuna-1.5} \cite{zheng2023judging} model as the large-language encoder. The feature alignment process was performed for 5k training steps with a learning rate of $1e-5$. The visual projector model learned from the feature alignment step is then used for instruction-tuning for predicting potential locations for the target object. The instruction-finetuning process is performed for 60k training steps with a learning rate of $1e-6$.

\subsection{Quantitative Experiments}
\label{sec:quantitative-experiments}

\textbf{Object Insertion.} In addition to qualitative results, we also report quantitative results comparing our approach to prior works \cite{rombach2021highresolution}  for object insertion.  To this end, we first collect a total of 8490 image-mask pairs where human users are shown a real image input and asked to provide a feasible  bounding box mask for inserting a target object (\eg dog) in the original image. The image-mask pairs along with the corresponding object description are then used to obtain object inpainting results for different baselines \cite{rombach2021highresolution,podell2023sdxl,avrahami2022blended}. The final scene context description $\mathcal{T}_{context}$ for \Smask is obtained by appending the object description in front of the scene-caption (obtained using InstructBLIP \cite{instructblip}) for the original image. The results for Adobe Smartbrush \cite{xie2023smartbrush} including both in-painted outputs as well as mask-head predictions (refer Sec.~\ref{sec:output-mask-quality}) are obtained directly from paper authors. The results for Adobe GenerativeFill \cite{adobe2023firefly} are obtained using the commercially available GenFill tool
from Adobe Firefly \cite{adobe2023firefly}. However, since no API for the same is available, quantiative results for GenFill (Table \textcolor{red}{1} main paper) are reported using a limited subset of 200 examples.

\textbf{Output Mask Quality.} 
% mask quality setting, number of samples, human subjects, and 
We also report quantitative results on output mask quality by comparing \Smask generated masks with SmartBrush \cite{xie2023smartbrush} mask-head predictions and different Inpaint+HQSAM methods (\ie inpainting first and then using HQSAM to obtain target object masks). To this end, we perform a human user study where given the input-image and object description, human subjects are shown a pair of object-insertion mask suggestions (ours vs baselines discussed above). For each pair, the human participant is then asked to select the object-mask suggestion with higher quality in terms of mask details, alignment with object description and mask realism/artifacts. The user-study data was performed among 50 human participants, who were given an unlimited time in order to ensure high quality of the final results. Additionally, in order to remove data noise, we use a repeated comparison (control seed) for each user. Responses of users who answer differently to this repeated seed are discarded while reporting the final results.

%-------------------------------------------------------------------------
% \newpage
\begin{figure*}[t]
% \vskip -0.15in
\begin{center}
\centerline{\includegraphics[width=1.\linewidth]{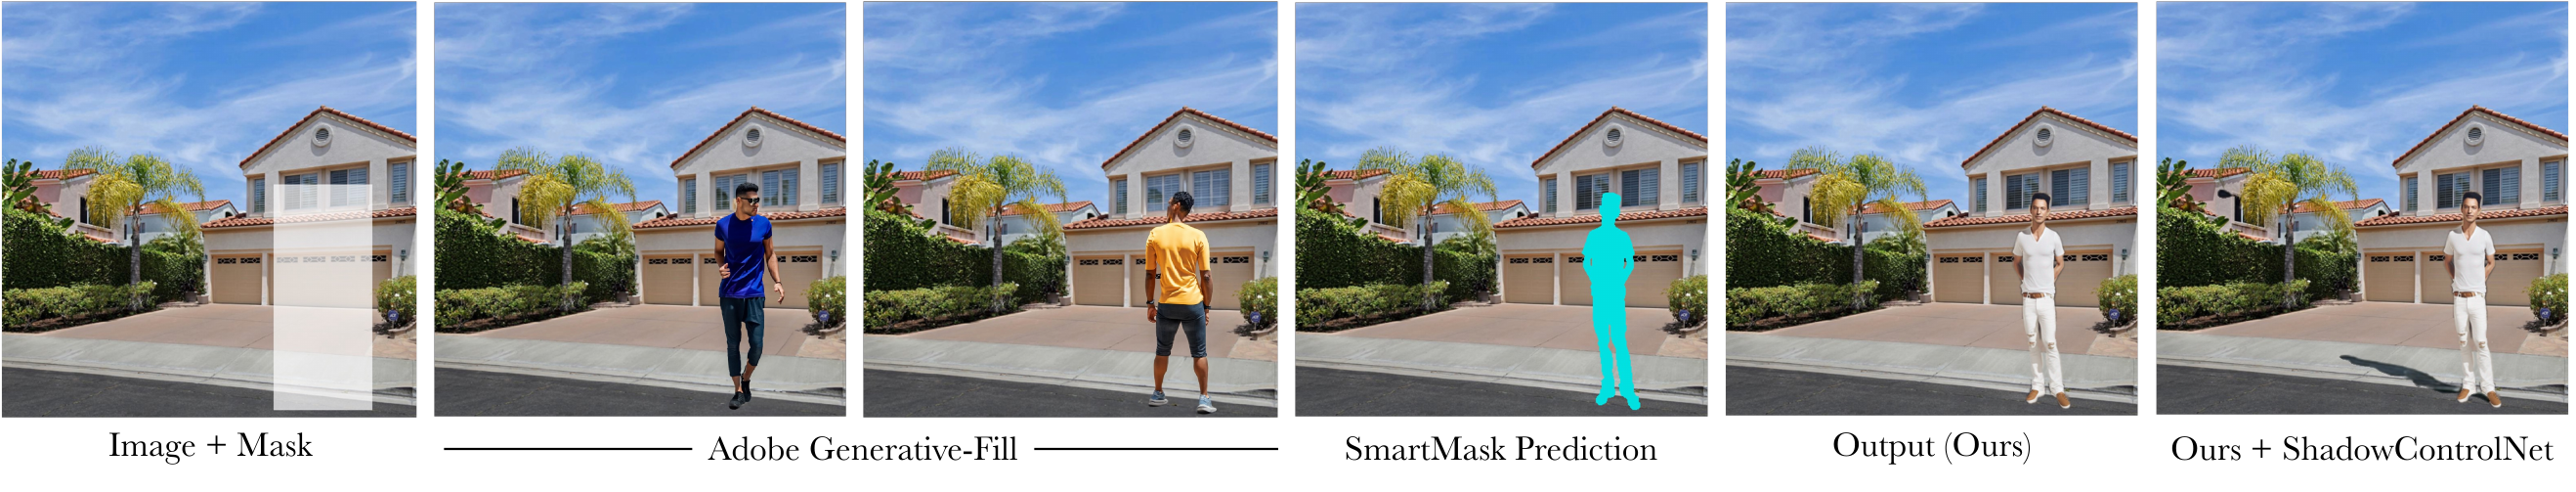}}
\vskip -0.1in
\caption{\emph{Shadow depiction.} We observe that shadow generation remains a challenging problem for even with most state-of-the-art image inpainting methods (\eg, Adobe GenFill \cite{adobe2023firefly} \emph{(left)} and Ours \emph{(right)}). Nevertheless, we find that the \Smask generated precise mask can be used as input to a second shadow-generation ControlNet model \cite{niu2021making} for better quality shadow generation for the inserted object. 
}
\label{fig:lim-shadow-generation}
\end{center}
\vskip -0.1in
\end{figure*}

\section{Additional Related Work}
\label{sec:related-work}

In addition to the related work discussed in Sec.~\textcolor{red}{2} of the main paper, the layout generation ability of the proposed approach can also be contrasted with bounding-box based specialized layout creation methods \cite{qu2023layoutllm,feng2023layoutgpt,zheng2019content,arroyo2021variational, gupta2021layouttransformer}. However, the generated layouts are represented by coarse bbox locations. In contrast, iterative use of the proposed \Smask model allows the user to control the scene layouts on a more finegrain level including object shape / structure, occlusion relationships, location \etc. Furthermore, as illustrated in Fig.~\textcolor{red}{7}b (main paper), we note that \Smask generated layouts are highly controllable and allow for a range of custom operations such as adding, removing, modifying or moving objects through simple layer manipulations.

%-------------------------------------------------------------------------
% \newpage
\section{Discussions and Limitations}
\label{sec:discussion}

While the proposed approach allows for better quality object insertion and layout control, it still has some limitations. \emph{First,} recall that current \Smask model is trained to predict object insertion suggestions based on the semantic layout $\mathcal{S}_I$ of the input image $\mathcal{I}$. While this 
allows us to leverage large-scale semantic amodal segmentation datasets \cite{qi2019amodal,zhu2017semantic} for obtaining high quality paired annotations during training,
% leads to competitive results, 
the use of semantic layout input for target mask prediction can be also be limiting as the semantic layout $\mathcal{S}_I$ typically has less depth context as opposed to the original image $\mathcal{I}$. In future, using a ControlNet generated S2I image as pseudo-label can help better train the model to directly predict the target object masks from the original image $\mathcal{I}$.

% generalization to out-of-dist data: success and failure case.
\emph{Second,} we note that in order to facilitate background preservation and mask-free object insertion, the current \Smask model is trained on a semantic amodal segmentation dataset consisting a total of 32785 diverse real world images (with $\sim 0.75$M different object instances). In contrast, typical object inpainting models such as Adobe SmartBrush \cite{xie2023smartbrush}, SDInpaint \cite{rombach2021highresolution,diffusers} are trained on datasets \cite{schuhmann2021laion} which are orders of magnitude larger in comparison (\eg Adobe SmartBrush \cite{xie2023smartbrush} and SDInpaint \cite{rombach2021highresolution} are trained on 600M samples from the LAION-Aesthetics-v2 5+ dataset \cite{schuhmann2021laion}).  While utilizing the generalizable prior of a pretrained Stable-Diffusion v1.5 model \cite{diffusers} allows our approach to generalize across diverse object categories (\eg mountains, waterfalls, building/towers, humans, dogs, cats, clouds, trees, furniture, electrical appliances \etc) with limited data, generating precise object masks for significantly out-of-distribution objects \eg, dragons remains challenging.  In future, the use of larger training datasets and stronger prior mode (SDXL \cite{podell2023sdxl}) can help alleviate this problem. 
% Furthermore, as shown in Fig.~\ref{fig:out-of-dist}, we note that LORA-finetuning the original \Smask model with a low-rank (4-8), on as few as 20-50 additional examples allows it to easily generalize to novel object categories.
% (\eg, dragons). 

\emph{Finally,} we note that similar to prior inpainting methods \cite{xie2023smartbrush, adobe2023firefly, podell2023sdxl,rombach2021highresolution}, 
accurate shadow-generation around the inserted object remains a challenging problem. For instance, in Fig.~
\ref{fig:lim-shadow-generation}, when adding a man in front of a house on a sunny day, we observe that both Adobe GenFill \cite{adobe2023firefly} and \Smask lead to limited shadow depiction around the inserted object. Nevertheless, we find that the \Smask generated precise mask can
be used as input to a second shadow-generation ControlNet model \cite{niu2021making} for better quality shadow generation for the inserted object.
That said, we note that precise shadow generation for the inserted object remains a challenging problem (with both prior work and ours). However, the same is out of scope of this paper, and we leave it
as a direction for future research.
